# Supplementary material for: Knight shifts, nuclear spin-relaxation rates, and spin echo decay times in the pseudogap regime of the cuprates: Simulation and relation to experiment
Source: arXiv:1607.05655 source file (2016-07-19)
Supplement: Supplementary file 1 [file supplemental.pdf]

# Supplemental material for: Knight shifts, nuclear spin-relaxation rates, and spin echo decay times in the pseudogap regime of the cuprates: Simulation and relation to experiment

Xi Chen,[1] J. P. F. LeBlanc,[1] and Emanuel Gull[1]

[1] *Department of Physics, University of Michigan, Ann Arbor, Michigan 48109, USA*

(Dated: July 19, 2016)

## GENERALIZED SUSCEPTIBILITY

We define the one-particle and two-particle Green's functions in imaginary time, $\tau$ as

$$G_\sigma(k_1\tau_1, k_2\tau_2) = \langle T_\tau(c^\dagger_{k_1\sigma}(\tau_1)c_{k_2\sigma}(\tau_2))\rangle \quad (1)$$

$$G_{2,\sigma_1\sigma_2\sigma_3\sigma_4}(k_1\tau_1, ..., k_4\tau_4) = \langle T_\tau(c^\dagger_{k_1\sigma}(\tau_1)c_{k_2\sigma}(\tau_2)c^\dagger_{k_3\sigma}(\tau_3)c_{k_4\sigma}(\tau_4))\rangle. \quad (2)$$

The generalized susceptibility can be written in imaginary time, $\tau$, in terms of the one- and two-particle Green's functions as [1]

$$\chi_{\sigma_1\sigma_2\sigma_3\sigma_4}(k_1\tau_1, k_2\tau_2, k_3\tau_3, k_4\tau_4) = G_{2,\sigma_1...\sigma_4}(k_1\tau_1, k_2\tau_2, k_3\tau_3, k_4\tau_4) - G_{\sigma_1\sigma_2}(k_1\tau_1, k_2\tau_2)G_{\sigma_3\sigma_4}(k_3\tau_3, k_4\tau_4).$$

The susceptibility can be represented in frequency space via a Fourier transform. In the particle-hole (ph) convention, it is defined as

$$\chi^{\omega\omega'\nu}_{ph\sigma\sigma'}(k, k', q) = \int_0^\beta \int_0^\beta \int_0^\beta d\tau_1 d\tau_2 d\tau_3 \chi_{\sigma\sigma\sigma'\sigma'}(k\tau_1, (k'+q)\tau_2, (k+q)\tau_3, k'0)e^{-i\omega\tau_1}e^{i(\omega+\nu)\tau_2}e^{-i(\omega'+\nu)\tau_3}$$

where $\omega$ and $\omega'$ are fermionic Matsubara frequencies, $\nu$ is a bosonic Matsubara frequency, $\sigma$ and $\sigma'$ are $\uparrow$ or $\downarrow$ spin labels and $k$, $k'$ and $q$ are initial, final and transfer momenta respectively. Spin susceptibility is the difference between the $\sigma\sigma' \equiv\uparrow\uparrow$ and $\uparrow\downarrow$.

$$\chi_m = \chi_{ph\uparrow\uparrow} - \chi_{ph\uparrow\downarrow}. \quad (3)$$

We define the bare susceptibility,

$$\chi^{\omega\omega'\nu}_{0ph}(k, k', q) = -\beta G_\sigma(k, i\nu)G_\sigma(q + k, i\nu + i\omega)\delta_{\omega\omega'}\delta_{kk'}, \quad (4)$$

where the spin index on the left hand side has been omitted when we restrict our calculation to the paramagnetic state. The Bethe-Salpeter equation in the magnetic channel is [1]

$$\chi^{\omega\omega'\nu}_m(k, k', q) = \chi^{\omega\omega'\nu}_{0ph}(k, k', q) - \frac{1}{\beta^2}\chi^{\omega\omega''\nu}_{0ph}(k, k'', q)\Gamma^{\omega''\omega'''\nu}_m(k'', k''', q)\chi^{\omega'''\omega'\nu}_m(k''', k', q). \quad (5)$$

where repeated indices are summed over and defines the vertex function $\Gamma$.

Within the DCA approximation [2], the single particle lattice self energy is coarse grained from its cluster counterpart, $\Sigma_\sigma(k, i\omega) = \Sigma_\sigma(K + \tilde{k}, i\omega) \approx \Sigma_\sigma(K, i\omega)$, where $K$ defines a cluster vector

and $\tilde{k}$ a vector within a momentum "patch".
Similarly the lattice susceptibility

$$\overline{\chi}_{0ph}^{\omega\omega'\nu}(K,K',Q) = -\beta\frac{N}{N_c}\sum_{\tilde{k}} G_\sigma(K+\tilde{k},i\nu)G_\sigma(Q+K+\tilde{k},i\nu+i\omega)\delta_{\omega\omega'}\delta_{KK'}, \tag{6}$$

Also, according to Fotso *et al.* [3], using $\Gamma = \frac{\delta\Sigma}{\delta G}$, perform an approximation on the vertex function.

$$\Gamma_m^{\omega\omega'\nu}(K,K',Q) = \Gamma_m^{\omega\omega'\nu}(K+\tilde{k},K'+\tilde{k'},Q+\tilde{q}) \to \Gamma_m^{\omega\omega'\nu}(K,K',Q). \tag{7}$$

We then sum over lattice momenta within one patch of k-space to get coarse-grain equation (5) as

$$\overline{\chi}_m^{\omega\omega'\nu}(K,K',Q) = \overline{\chi}_{0ph}^{\omega\omega'\nu}(K,K',Q) - \frac{1}{\beta^2}\overline{\chi}_{0ph}^{\omega\omega''\nu}(K,K'',Q)\Gamma_{cm}^{\omega''\omega'''\nu}(K'',K''',Q)\overline{\chi}_m^{\omega'''\omega'\nu}(K''',K',Q). \tag{8}$$

Cluster quantities also follow the Bethe-salpeter equation,

$$\chi_m^{\omega\omega'\nu}(K,K',Q) = \chi_{0cph}^{\omega\omega'\nu}(K,K',Q) - \frac{1}{\beta^2}\chi_{c0ph}^{\omega\omega''\nu}(K,K'',Q)\Gamma_{cm}^{\omega''\omega'''\nu}(K'',K''',Q)\chi_{cm}^{\omega'''\omega'\nu}(K''',K',Q). \tag{9}$$

One then combines equations (8) and (9) to eliminate the cluster vertex, $\Gamma_c$, to obtain

$$\overline{\chi}^{-1} = \chi_c^{-1} - \chi_{0c}^{-1} + \overline{\chi}_0^{-1} \tag{10}$$

where $\overline{\chi}$, $\chi_c$, $\chi_{0c}$ and $\overline{\chi}_0$ are all matrices in cluster momentum $K$ and frequency $\omega$. This procedure is described in detail in Ref. [2].

## NMR RELATED QUANTITIES: $K^S$, $T_{2g}$ AND $T_1$

One quantity of interest is the spin-lattice relaxation rate $1/T_1$. It is related to the imaginary part of dynamical spin susceptibility on the real frequency axis.

$$\frac{1}{T_1T} \propto \lim_{\nu\to 0}\sum_q {}^{\alpha}F_{\parallel}(q)\frac{\chi_m''(q,\nu)}{\nu} \tag{11}$$

where ${}^{\alpha}F_{\parallel}(q)$ differs for ${}^{63}Cu$ and ${}^{17}O$, as defined in Ref. [4]. These are

$$\begin{aligned} {}^{63}F_{\parallel} &= A_\perp + 2B[\cos(q_x)+\cos(q_y)]^2 \\ {}^{17}F_{\parallel} &= 2C_{\parallel}^2[1+0.5[\cos(q_x)+\cos(q_y)]] \\ A_\perp &= 0.84B, C_{\parallel} = 0.91B. \end{aligned} \tag{12}$$

Obtaining $\chi_m''(q,\nu)/\nu$ typically requires analytical continuation. If temperature is low enough, we can consider the parametrization

$$\chi_m''(q,\nu) = \nu\chi_m(q,0)/\Gamma_q. \tag{13}$$

We can then write the spin structure factor, $S(q,\tau)$ at time $\tau=\beta/2$ as

$$S(q,\tau=\frac{\beta}{2})=\int d\nu\frac{\chi_m(q,0)\nu}{\Gamma_q\sinh\frac{\nu}{2T}}=\frac{\chi_m(q,0)}{\Gamma_q}\int\frac{4T^2\lambda d\lambda}{\sinh\lambda}=T^2\pi^2\frac{\chi_m(q,0)}{\Gamma_q}\tag{14}$$

where $S(q,\tau)=\langle s_q^z(\tau)s_{-q}^z(0)\rangle$ and $S_q^z$ is the real-to-k-space Fourier transform of $s_i^z=n_{i\uparrow}-n_{i\downarrow}$. To connect $S(q,\tau)$ with spin susceptibility,

$$\begin{aligned}S(q,\tau)=\langle s_q^z(\tau)s_{-q}^z(0)\rangle&=\frac{1}{N}\langle\sum_{R_iR_j}e^{-iq(R_i-R_j)}\times[n_{i\uparrow}(\tau)-n_{i\downarrow}(\tau)][n_{j\uparrow}(0)-n_{j\downarrow}(0)]\rangle\\&=\frac{1}{N}\langle\sum_{R_iR_j}e^{-iq(R_i-R_j)}\times[c^\dagger_{i\uparrow}c_{i\uparrow}c^\dagger_{j\uparrow}c_{j\uparrow}-c^\dagger_{i\downarrow}c_{i\downarrow}c^\dagger_{j\uparrow}c_{j\uparrow}-c^\dagger_{i\uparrow}c_{i\uparrow}c^\dagger_{j\downarrow}c_{j\downarrow}+c^\dagger_{i\downarrow}c_{i\downarrow}c^\dagger_{j\downarrow}c_{j\downarrow}]\rangle\end{aligned}\tag{15}$$

where we have omitted $\tau$ in the equation. Note that creation/annihilation operator site $i$ has imaginary time $\tau$ and site $j$ $\tau=0$.

$$\frac{1}{\sqrt{N}}\sum_q c_q e^{iqR_i}=c_i,\ \frac{1}{\sqrt{N}}\sum_q c_q^\dagger e^{-iqR_i}=c_i^\dagger\tag{16}$$

Omit spin indices for now, terms in equation 15 becomes

$$\frac{1}{N^3}[\sum_{k_1k_2}(\sum_{R_i}e^{iR_i(-q+k_1-k_2)})c^\dagger_{k_1}c_{k_2}][\sum_{p_1p_2}(\sum_{R_j}e^{iR_j(q+p_1-p_2)})c^\dagger_{p_1}c_{p_2}]\quad=\frac{1}{N}\sum_{k_2}c^\dagger_{k_2+q}c_{k_2}\sum_{p_2}c^\dagger_{p_2-q}c_{p_2}\tag{17}$$

There are four terms like this, with spin ↑↑↑↑, ↓↓↑↑, ↑↑↓↓, ↓↓↓↓ separately. Given the symmetry of 2 particle green's function, we then add imaginary time back and find

$$S(q,\tau)=\frac{1}{N}\langle(2\sum_{kk'}c^\dagger_{k+q\uparrow}(\tau)c_{k\uparrow}(\tau)c^\dagger_{k'\uparrow}(0)c_{k'+q\uparrow}(0)\tag{18}$$

$$-2\sum_{kk'}c^\dagger_{k+q\uparrow}(\tau)c_{k\uparrow}(\tau)c^\dagger_{k'\downarrow}(0)c_{k'+q\downarrow}(0))\rangle\tag{19}$$

where $k=k_2$, $k'=p_2-q$. This is the magnetic channel susceptibility. So

$$S(q,\tau)=\frac{1}{N}\sum_{kk'}\chi_m(k+q,\tau;k,\tau;k',0;k'+q,0)=\frac{2}{N}\sum_{kk'}\chi_m^{kk'q}(\tau,\tau,0)\tag{20}$$

Fourier transform it to Matsubara frequency space, get

$$S(q,\tau)=\frac{2}{N\beta^3}\sum_{kk',\omega\omega'\nu}\chi_m^{\omega\omega'\nu}(k,k',q)e^{-i\nu\tau}\tag{21}$$

With DCA,

$$\sum_q{}^\alpha F_\parallel(q)S(q,\tau)=\frac{2}{N\beta^3}(\frac{N}{N_c})^3\sum_{KK'Q}\sum_{\omega\omega'\nu}{}^\alpha F_\parallel(Q)\chi_m^{\omega\omega'\nu}(K,K',Q)e^{-i\nu\tau}=\frac{2}{\beta}\sum_{Q,\nu}{}^\alpha F_\parallel(Q)\chi_m(Q,i\nu)e^{-i\nu\tau}\tag{22}$$

Combine Eq. 13, Eq. 14 and Eq. 22

$$\frac{1}{T_1} = \frac{\sum_q {}^{\alpha}F_{\|}(q)S(q,\tau=\beta/2)}{\pi^2 T} = \frac{2}{\beta\pi^2 T}\sum_{Q,\nu} {}^{\alpha}F_{\|}(Q)\chi_m(Q,i\nu)e^{-i\nu\beta/2} \tag{23}$$

$$= \frac{2}{\pi^2}\sum_{Q,n} {}^{\alpha}F_{\|}(Q)\chi_m(Q,i\nu_n)(-1)^n \tag{24}$$

According to the Mila-Rice-Shastry model for HF coupling with itinerant $Cu^{2+}$ holes in high Tc cuprates, the Knight shift $K^S$ is proportional to uniform spin susceptibility $\chi_m(Q=0,\nu=0)$. For example, According to Ref[4], in $YBa_2Cu_3O_7$

$$\begin{aligned} {}^{63}K^S_{\|} &= \frac{A_{\|}+4B}{{}^{63}\gamma_n\gamma_e\hbar^2}\chi_m(Q=0,\nu=0), \quad {}^{63}K^S_{\perp} = \frac{A_{\perp}+4B}{{}^{63}\gamma_n\gamma_e\hbar^2}\chi_m(Q=0,\nu=0), \\ {}^{17}K^S_{\beta} &= \frac{A_{\perp}+4B}{{}^{17}\gamma_n\gamma_e\hbar^2}\chi_m(Q=0,\nu=0), \quad {}^{89}K^S = \frac{A_{\perp}+4B}{{}^{89}\gamma_n\gamma_e\hbar^2}\chi_m(Q=0,\nu=0), \end{aligned} \tag{25}$$

${}^{63}K^S_{\|}$, ${}^{63}K^S_{\perp}$, ${}^{17}K^S_{\beta}$, and ${}^{89}K^S$ are all proportional to $\chi_m(Q=0,\nu=0)$, with different ratios determined by the on-site coupling strength and transferred hyperfine coupling strength of $Cu^{2+}$ spin to ${}^{63}Cu$, ${}^{17}O$ and ${}^{89}Y$ nuclei. Here indices $\|$ and $\perp$ refer to the direction of the static magnetic field. $A_{\|}$, $A_{\perp}$, $B$, $C_{\beta}$ and $D$ are hyperfine coupling constants.
As for the ${}^{63}Cu$ nuclear spin echo decay rate $1/({}^{63}T_{2G})$ in the paramagnetic state of high $T_c$ cuprates, Pennington and Slichter [5] showed that

$${}^{63}T_{2G}^{-2} = \frac{0.69}{128\hbar^2}\left[\frac{1}{N}\sum_Q {}^{63}F_{eff}(Q)^2\chi'_m(Q,0)^2 - \left(\frac{1}{N}\sum_Q {}^{63}F_{eff}(Q)\chi'_m(Q,0)\right)^2\right], \tag{26}$$

where $\chi'_m(Q,0)$ is the real part of the dynamical spin susceptibility at momentum $Q$ and frequency 0. ${}^{63}F_{eff}(Q)$ is defined in Ref. 4 as

$${}^{63}F_{eff} = \{A_{\|} + 2B[cos(Q_x a) + cos(Q_y a)]\}^2 \tag{27}$$

$$A_{\|} = -4B. \tag{28}$$

We can extract the susceptibility $\chi'_m(Q,\nu=0)$ at real frequency $\nu=0$ from the DCA calculation result on the imaginary frequency axis, using $\chi'_m(Q,\nu=0) = \chi_m(Q,i\nu=0)$.

## SPECTRAL FUNCTION

See Fig. S1 for analytically continued spectral functions.

## SPIN LATTICE RELAXATION RATE $T_1^{-1}$

Fig. S2 shows that DCA and RPA calculation agrees at small interaction, low temperature region. Their discrepancy at higher temperature is expected. As explained in Eq.8 in the main text, the approximation of $\frac{1}{T_1}$ is better at low temperature.

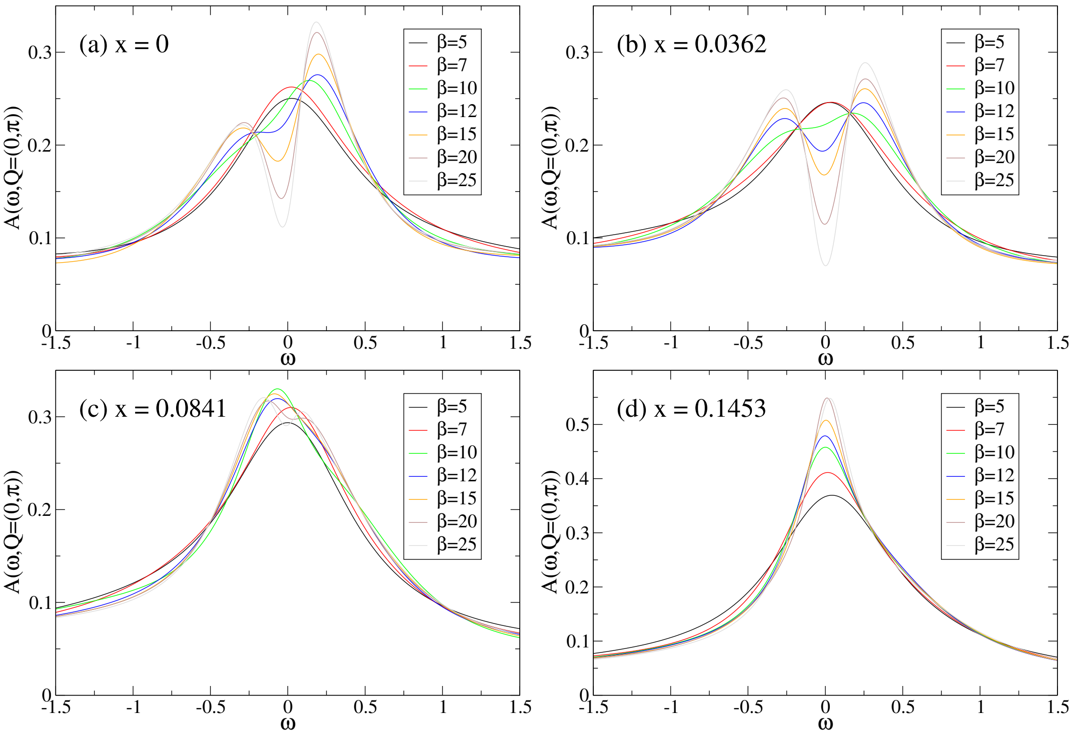


FIG. S1. Spectral function $A(\omega, Q = (0, \pi))$ for 8 site Hubbard model with $U = 6t$, $t' = -0.1t$, $x = 0, 0.0362, 0.0831, 0.1453$, obtained using DCA and Maxent.

Fig. S3 shows T- and doping-dependence of $(T_1)^{-1}$ of $^{63}Cu$ for 3 doping levels. It increase with reduced temperature at 0 doping. Towards larger hole doping, it becomes smaller and evolves to a curve that bent down at low temperature. These features agree with $LSCOx$ experiment at low temperature region (Fig.3 in Ref. [6],Fig.2 in [7]). At higher temperature $(T_1)^{-1}$ is temperature independent in experiment. But the approximation made in Eq.8 in main text prevent us from getting accurate $(T_1)^{-1}$ in this region.

According to Eq. 17, to get $T_1^{-1}$, one needs to sum bosonic frequency $\nu$ from 0 to $\infty$. However, the computation time grows as $\nu^3$. Although $\chi(i\nu)$ decays rapidly, the realistic cut-off frequency $\frac{2\pi n}{\beta}$ are insufficient at low temperature. As plotted in Fig. S5, the high frequency behavior $\chi(i\nu)$ are almost the same for different temperatures, attaching the high frequency tail to the truncated low temperature curve is a method to compensate for its summation. We first do a polynomial fitting to the $\beta = 5$ curve, then using this fitted tail as an estimation of high frequency $\chi(i\nu)$ for lower temperatures. The error bars are estimated based on the discrepancy of the fitted polynomial and actual $\chi_m$, which we believe yields the largest contribution to the error, and do not include other sources of error. Note in particular that the numerical error of $\chi(Q, i\nu)$ is not included.

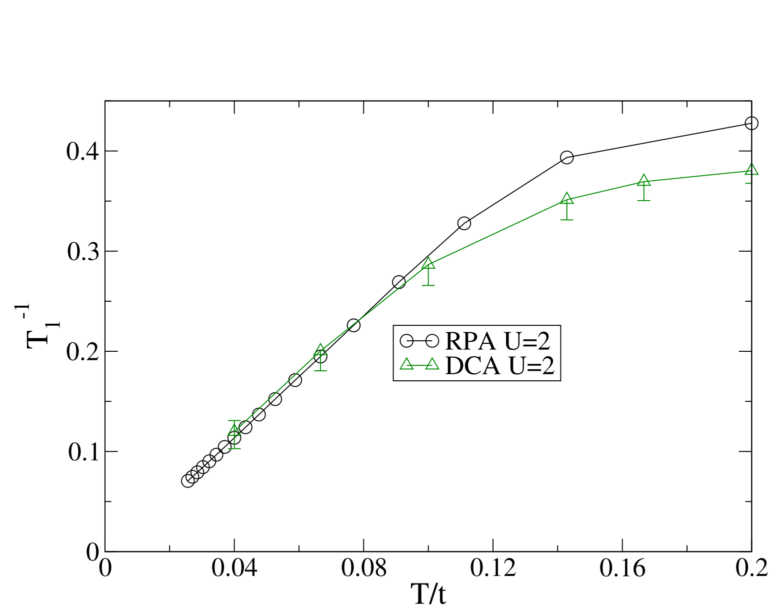


FIG. S2. Spin lattice decay rate of 8-site Hubbard model at $U = 2t$, $t' = 0$. Black solid line, open circle symbol: RPA results. Green solid line with error bar: DCA results.


[1] G. Rohringer, A. Valli, and A. Toschi, Phys. Rev. B **86**, 125114 (2012).
[2] T. Maier, M. Jarrell, T. Pruschke, and M. H. Hettler, Rev. Mod. Phys. **77**, 1027 (2005).
[3] H. Fotso, S. Yang, K. Chen, S. Pathak, J. Moreno, M. Jarrell, K. Mikelsons, E. Khatami, and D. Galanakis, *Dynamical Cluster Approximation* (Springer-Verlag Berlin Heidelberg, 2012).
[4] V. Barzykin and D. Pines, Phys. Rev. B **52**, 13585 (1995).
[5] C. H. Pennington and C. P. Slichter, Phys. Rev. Lett. **66**, 381 (1991).
[6] S. Ohsugi, Y. Kitaoka, K. Ishida, G. qing Zheng, and K. Asayama, Journal of the Physical Society of Japan **63**, 700 (1994).
[7] T. Imai, C. P. Slichter, K. Yoshimura, and K. Kosuge, Phys. Rev. Lett. **70**, 1002 (1993).

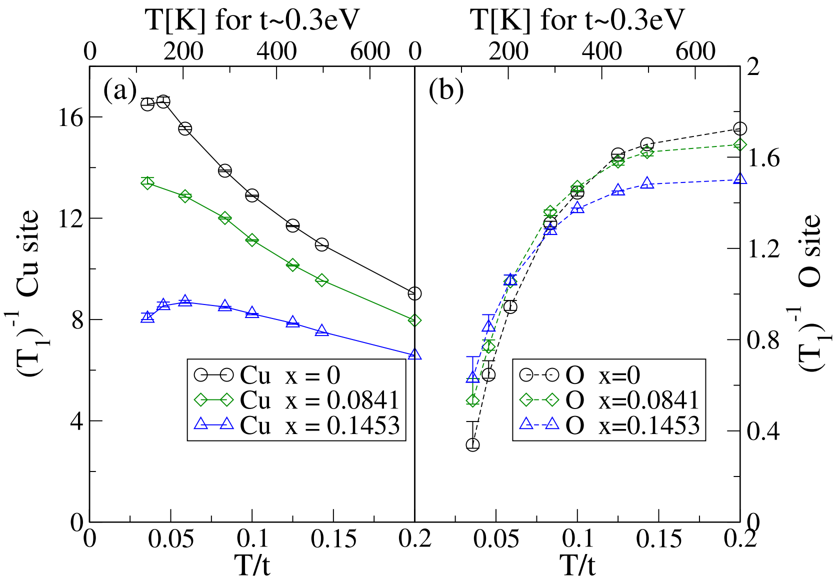


FIG. S3. $(T_1)^{-1}$ plotted as a function of temperature at $U = 6t$, $t' = -0.1t$, for $x = 0$ to $x = 0.145$, by 8-site DCA. Panel (a), solid lines: symmetry factors corresponding to $^{63}Cu$ site. Panel (b), dashed line: $^{17}O$ site.

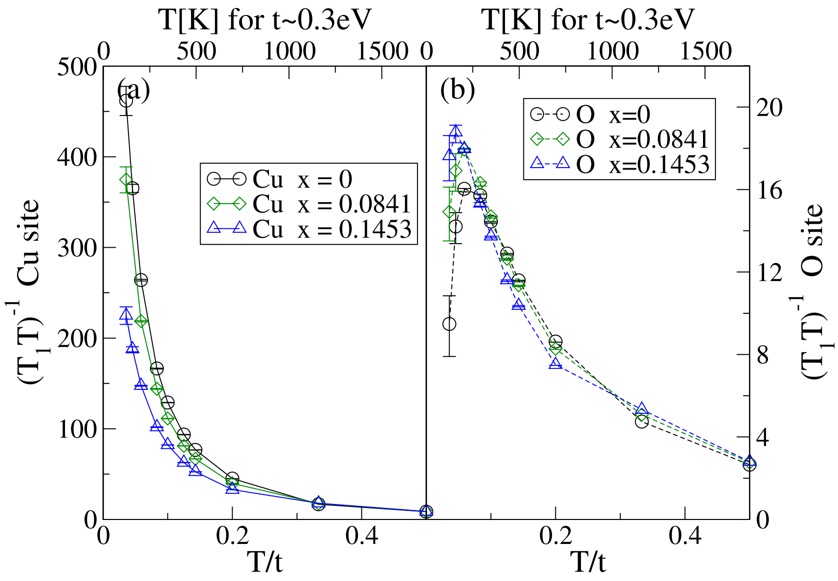


FIG. S4. $(T_1T)^{-1}$ plotted as a function of temperature at $U = 6t$, $t' = -0.1t$, for $x = 0$ to $x = 0.145$ extended to higher temperature, by 8-site DCA. Panel (a), solid lines: symmetry factors corresponding to $^{63}Cu$ site. Panel (b), dashed line: $^{17}O$ site.

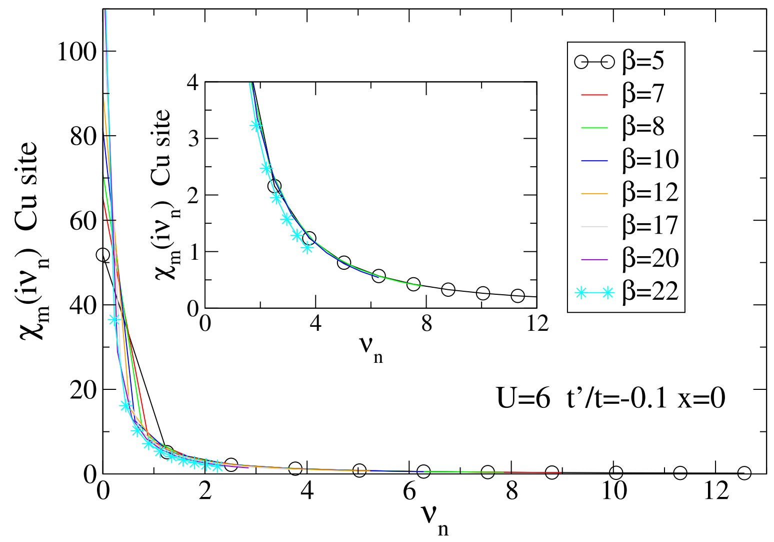


FIG. S5. Spin susceptibility on Matsubara frequency of 8-site Hubbard model at $U = 6t$, $t' = -0.1t$ at different temperature.
